# Supplementary material for: Captured by Captions: On Memorization and its Mitigation in CLIP Models
Source: arXiv:2502.07830 source file (2025-05-19)
Supplement: Supplementary file 1 [file appendix_not_include.tex]

\begin{figure}[t]
    \centering
    \includegraphics[width=0.95\linewidth]{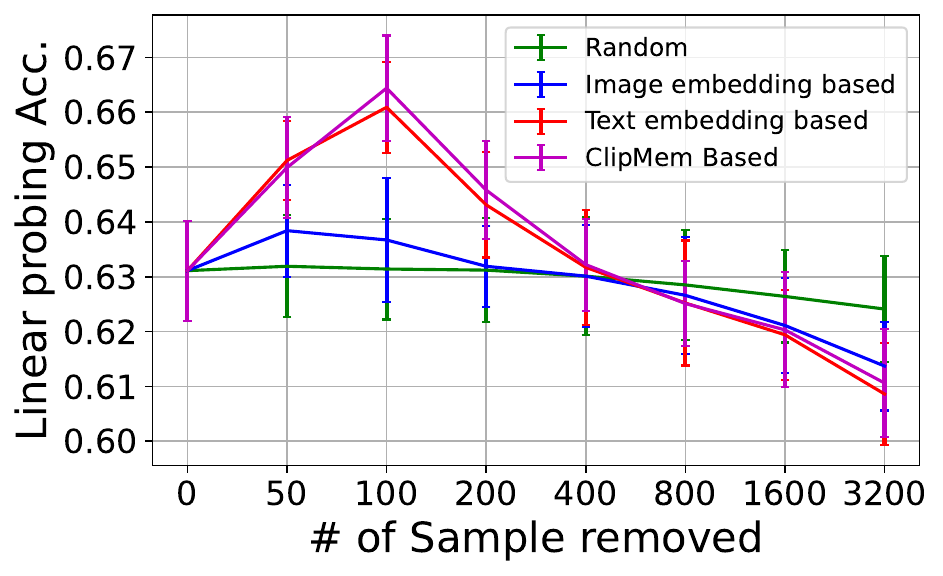}
    \caption{\textbf{Removing memorized samples}we can see the results of text-based is much closer to the ClipMem-based, while ClipMem-based has a even better effect}
    \label{fig:image_sample_remove_whole}
\end{figure}

Furthermore, we present the overlap in the number of samples reported as memorized by SSLMem on the different modalities with the highest 500 memorized samples reported by CLIPMem, see for example \Cref{fig:examples}.
In total SSLMem on the vision encoder identifies 105/500 samples that are highly memorized according to CLIPMem, whereas SSLMem identifies 143/500 samples when applied to the text encoder.
The overlap between the 500 samples reported as highly memorized by SSLMem on the text and on the image encoder is 389/500. This again indicates that using only SSLMem on an individual modality is insufficient. 
\adam{However, it even leads to different samples being selected by CLIPMem vs SSLMem while the overlap between the selected data points by SSLMem for vision and text encoder is quite substantial.}
\textcolor{red}{This indicates that...}

\begin{figure}[t]
    \centering
    \includegraphics[width=0.55\linewidth]{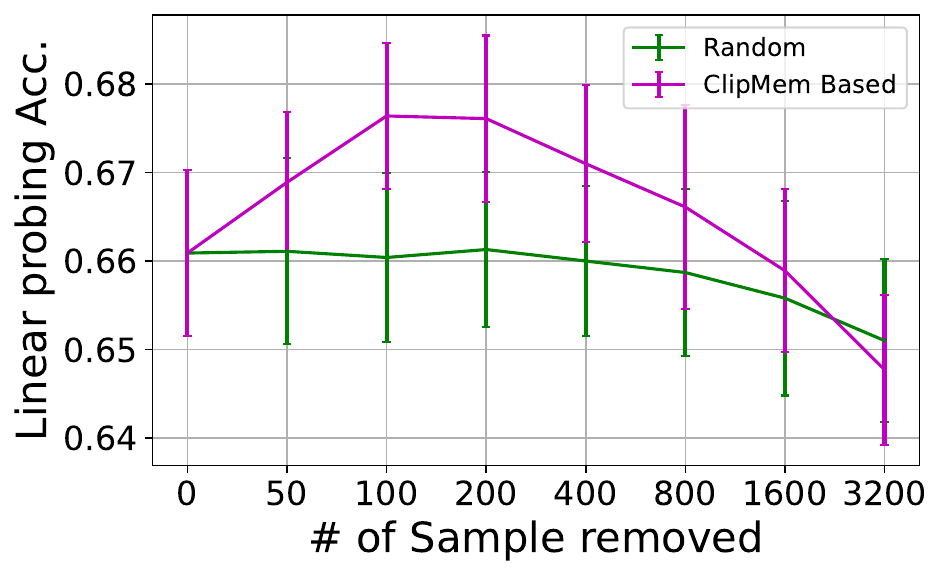}
    \caption{\textbf{Removing memorized samples for CC3M.} We use 65000 samples as $S_S$, 5000 as $S_C$, and 5000 as $S_I$. 
    %random samples (random picked and generate a list for them, could be resued in future) 
    The samples are selected at random out of 2.91M total number of data points in the CC3M dataset~\citep{sharma2018conceptual}.}
    \label{fig:image_text_sample_cc3m}
\end{figure}

\subsubsection{Studying Memorization per Modality}
\label{app:modality}
\todo{@Adam, I find it very hard to justify the experiment below. Can you please have a look? The reviewers might just be confused.}
We also perform an experiment where we remove memorized samples, retrain the model, and report the resulting linear probing accuracy.
The more the linear probing accuracy is affected by the removal of a memorized sample, the more important the samples.
Rather than taking the overall highest memorized samples and removing them, once the model is trained, we first cluster the training data in the embedding space into 50 clusters, once according to the text and once according to the image embeddings.
Then, we remove from each cluster the highest memorized data point.
This semantically corresponds to finding the highest memorized data points per-class in supervised learning (with the difference that we have no class information, and therefore, have to revert to a default number of clusters, in our case 50).
Our results in \Cref{fig:modality} highlight that removing the highest memorized samples according to the text embeddings' grouping and then re-training boosts downstream performance more than removing based on image embeddings.\todo{@Adam, here, for sure something is missing, an explanation or so. But I have none. In the worst case, we need to remove this paragraph.} 
Hence, the overall observed trend indicates that memorization in CLIP depends more on the text than on the image.
\begin{figure}[h]
    \centering
    \includegraphics[width=0.55\linewidth]{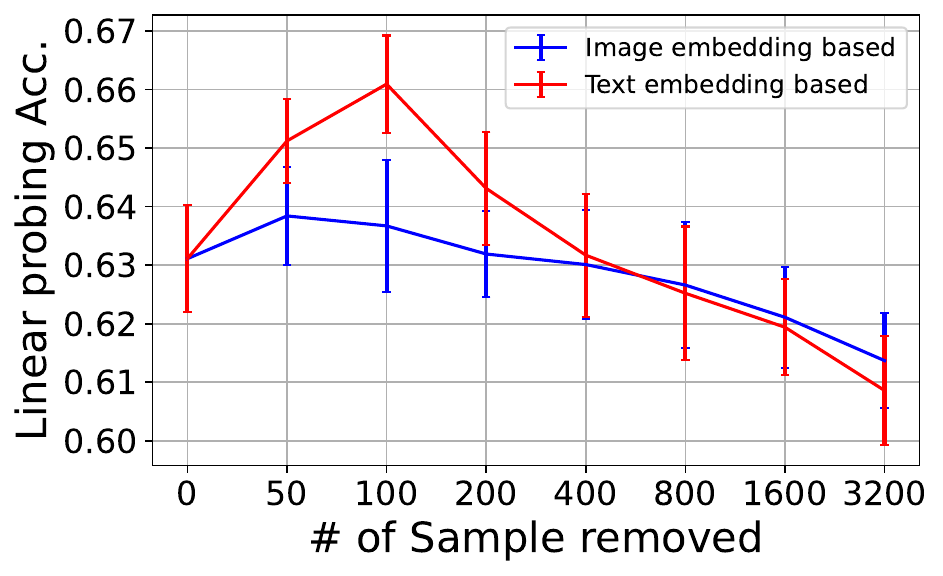}
    \caption{\textbf{Modality-based removal.} We train a CLIP models with standard image cropping on the COCO dataset. 
    After training, we cluster training samples according to their similarity based on CLIP's image or text embeddings into 50 clusters, remove the highest memorized sample from each cluster, and retrain with the remaining points. The linear probing accuracy on ImageNet suggests that removing based on text embeddings' clustering memorization has higher influence on model performance.}
    \label{fig:modality}
\end{figure}

\subsection{Regrouping}
\begin{table}[t]
          \caption{\textbf{Experiment for applying regrouping during training.} For each 10 epoch (out of 100), we regrouping all samples into batches according their pairwise cos-similarities. Inside each batch, the representation of samples' caption are as similar to each other as possible.}        
          \label{tab:reduce_memorization}
    \centering
    \scriptsize
    \scalebox{0.85}{\begin{tabular}{ccccc}
    \toprule
&Baseline & Retrain based on & Memorization-regrouping & K-mean balanced \\
&&memorization&during training &during training \\
    \midrule
Avg. CLIPMem (Top 128) & 0.761&0.692&0.671&0.679\\
Avg. CLIPMem (Top 20\%) &0.552&0.514&0.541&0.533\\
Avg. CLIPMem &0.438&0.409&0.433&0.432\\
LP. Acc. & 63.11\% $\pm$ 0.91\%& 60.23\% $\pm$ 1.12\% &62.09\% $\pm$ 0.96\% &62.98\% $\pm$ 1.00\%\\
      \bottomrule     
      \end{tabular}}
\end{table}
We additionally experimented with a different strategy to reduce memorization.
We observed that CLIP's training objective which maximizes the dot product of the representations for matching image-caption pairs within the same batch while minimizing the dot product of the representations of unrelated image-caption pair helps eliminate the impact of "mis-captioned" samples on memorization.
\textcolor{red}{@Wenhao, what was the intuition why the regrouping should work?}
Based on this observation, we performed multiple experiments.
As a \textit{Baseline}, we take a standard OpenCLIP model trained by COCO with only one caption.
Then, after training, we use this model and measure our \ours scores. 
We group the samples into mini-batches according to their experienced memorization, \ie highly memorized samples are in the same batch as other highly memorized samples, and we retrain with this new grouping of data points by setting random shuffle in the data loader to 'off' (\textit{Retrain based on memorization}). 
Additionally, to avoid having to retrain from scratch, we apply mini-batch re-grouping every 10 epochs during training:
For the first case, we re-group again according to memorization every 10 epochs (\textit{Memorization-regrouping during training}), and finally, we re-group during training, but according to semantic similarity in the text domain.
Therefore, we obtain all training data's text embeddings and apply the balanced k-mean algorithm with as many clusters as training mini-batches (\textit{K-mean balanced during training}).
Our results in \Cref{tab:reduce_memorization} highlight that these strategies can slightly reduce memorization but also at the cost of utiliyt.
